# Supplementary material for: OntoED: Low-resource Event Detection with Ontology Embedding
Source: arXiv:2105.10922 source file (2022-04-04)
Supplement: Supplementary file 1 [file appendix.tex]

\section{Appendices}
\label{sec:appendices}

Here we list detailed statistics of \texttt{OntoEvent}.

\subsection{Hierarchical Event Type Schema}

\input{tables/Table_Hierarchical-Event-Types}

\clearpage

\subsection{Overview of Temporal \& Causal Event-Event Correlations}

\input{tables/Table_Event-Event-Correlations}

% \clearpage
